# Supplementary material for: When are Post-hoc Conceptual Explanations Identifiable?
Source: arXiv:2206.13872 source file (2023-06-06)
Supplement: Supplementary file 1 [file cub_appendix.tex]

% \documentclass{article}

% \usepackage{graphicx}
% \usepackage{tikz}

% \begin{document}
\begin{tikzpicture}
% \draw[<->,thick] (p1.south east) -- (p2.north west)
%     node[midway,fill=white] {Principia Mathematica};

\newcommand{\tabspace}[0]{1.3}
\newcommand{\offset}[0]{2}
\newcommand{\imgw}[0]{.08\linewidth}
\newcommand{\textoffset}[0]{0.7}
\newcommand{\secoffset}[0]{-1.7}
    
\node[inner sep=0pt] (n1) at (-\offset,0)
    {\includegraphics[width=\imgw]{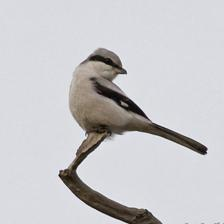}};
\node at (-1*\offset, \textoffset) {\tiny{0.0}};

\node[inner sep=0pt] (n2) at (-1*\tabspace-\offset,0)
    {\includegraphics[width=\imgw]{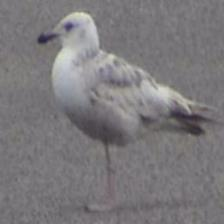}};
\node at (-1*\tabspace-\offset, \textoffset) {\tiny{0.0}};

\node[inner sep=0pt] (n3) at (-2*\tabspace-\offset,0)
    {\includegraphics[width=\imgw]{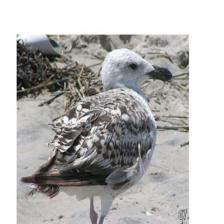}};
\node at (-2*\tabspace-\offset, \textoffset) {\tiny{0.0}};
    
\node[inner sep=0pt] (n4) at (-3*\tabspace-\offset,0)
    {\includegraphics[width=\imgw]{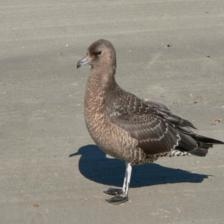}};
\node at (-3*\tabspace-\offset, \textoffset) {\tiny{0.0}};

\node[inner sep=0pt] (n5) at (-4*\tabspace-\offset,0)
    {\includegraphics[width=\imgw]{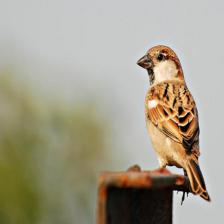}};
\node at (-4*\tabspace-\offset, \textoffset) {\tiny{0.0}};

\node at (-0.5*\offset, 0) {...};
\node at (-0.5*\offset, -1*\textoffset) {\tiny{Nape color: Olive}};

\draw [-latex](0.01*\offset, -1*\textoffset) -- (5.7, -1*\textoffset);
\node at (5.9, -1*\textoffset) {{\tiny{$+$}}};
\draw [-](-1*\offset, -1*\textoffset) -- (-7.7, -1*\textoffset);
\node at (-7.9, -1*\textoffset) {{\tiny{$-$}}};

% \node[inner sep=0pt] (n2) at (-5*\tabspace-\offset,0)
%     {\includegraphics[width=\imgw]{3.jpg}};

\node[inner sep=0pt] (p1) at (0,0)
    {\includegraphics[width=\imgw]{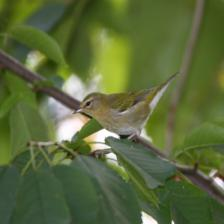}};
\node at (0, \textoffset) {\tiny{17.31}};

\node[inner sep=0pt] (p2) at (\tabspace,0)
    {\includegraphics[width=\imgw]{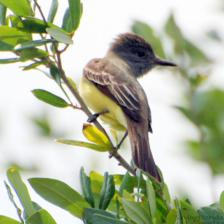}};
\node at (\tabspace, \textoffset) {\tiny{3.97}};

\node[inner sep=0pt] (p3) at (2*\tabspace,0)
    {\includegraphics[width=\imgw]{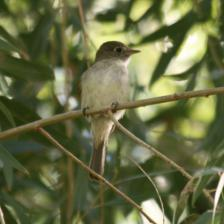}};
\node at (2*\tabspace, \textoffset) {\tiny{3.17}};
    
\node[inner sep=0pt] (p4) at (3*\tabspace,0)
    {\includegraphics[width=\imgw]{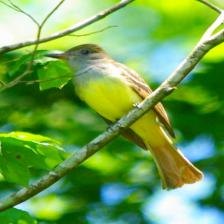}};
\node at (3*\tabspace, \textoffset) {\tiny{3.97}};

\node[inner sep=0pt] (p5) at (4*\tabspace,0)
    {\includegraphics[width=\imgw]{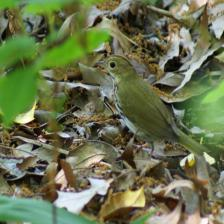}};
\node at (4*\tabspace, \textoffset) {\tiny{17.99}};

%%%%%% one more example
\node[inner sep=0pt] (n1) at (-\offset,\secoffset)
    {\includegraphics[width=\imgw]{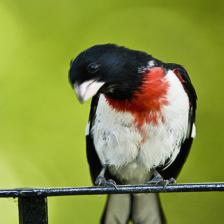}};
\node at (-1*\offset, \secoffset+\textoffset) {\tiny{1.96}};

\node[inner sep=0pt] (n2) at (-1*\tabspace-\offset,\secoffset)
    {\includegraphics[width=\imgw]{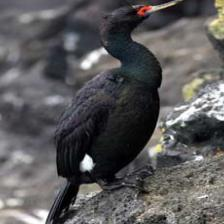}};
\node at (-1*\tabspace-\offset, \textoffset+\secoffset) {\tiny{0.0}};

\node[inner sep=0pt] (n3) at (-2*\tabspace-\offset,\secoffset)
    {\includegraphics[width=\imgw]{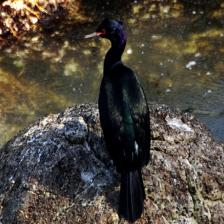}};
\node at (-2*\tabspace-\offset, \textoffset+\secoffset) {\tiny{3.16}};
    
\node[inner sep=0pt] (n4) at (-3*\tabspace-\offset,\secoffset)
    {\includegraphics[width=\imgw]{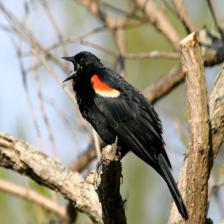}};
\node at (-3*\tabspace-\offset, \textoffset+\secoffset) {\tiny{0.0}};

\node[inner sep=0pt] (n5) at (-4*\tabspace-\offset,\secoffset)
    {\includegraphics[width=\imgw]{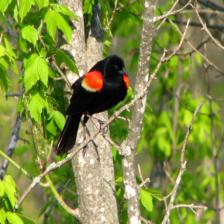}};
\node at (-4*\tabspace-\offset, \textoffset+\secoffset) {\tiny{0.0}};

\node at (-0.5*\offset, \secoffset) {...};
\node at (-0.5*\offset, -1*\textoffset+\secoffset) {\tiny{Back color: Buff}};

\draw [-latex](0.01*\offset, -1*\textoffset+\secoffset) -- (5.7, -1*\textoffset+\secoffset);
\node at (5.9, -1*\textoffset+\secoffset) {{\tiny{$+$}}};
\draw [-](-1*\offset, -1*\textoffset+\secoffset) -- (-7.7, -1*\textoffset+\secoffset);
\node at (-7.9, -1*\textoffset+\secoffset) {{\tiny{$-$}}};

% \node[inner sep=0pt] (n2) at (-5*\tabspace-\offset,0)
%     {\includegraphics[width=\imgw]{3.jpg}};

\node[inner sep=0pt] (p1) at (0,\secoffset)
    {\includegraphics[width=\imgw]{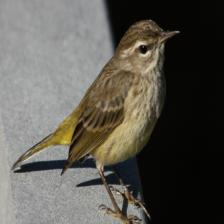}};
\node at (0, \textoffset+\secoffset) {\tiny{42.11}};

\node[inner sep=0pt] (p2) at (\tabspace,\secoffset)
    {\includegraphics[width=\imgw]{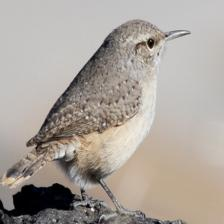}};
\node at (\tabspace, \textoffset+\secoffset) {\tiny{49.63}};

\node[inner sep=0pt] (p3) at (2*\tabspace,\secoffset)
    {\includegraphics[width=\imgw]{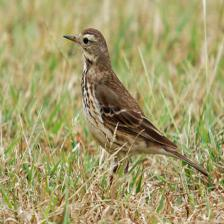}};
\node at (2*\tabspace, \textoffset+\secoffset) {\tiny{53.42}};
    
\node[inner sep=0pt] (p4) at (3*\tabspace,\secoffset)
    {\includegraphics[width=\imgw]{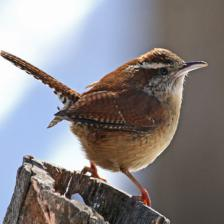}};
\node at (3*\tabspace, \textoffset+\secoffset) {\tiny{19.58}};

\node[inner sep=0pt] (p5) at (4*\tabspace,\secoffset)
    {\includegraphics[width=\imgw]{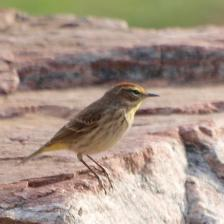}};
\node at (4*\tabspace, \textoffset+\secoffset) {\tiny{42.11}};

%%%%%% one more example

\node[inner sep=0pt] (n1) at (-\offset, 2*\secoffset)
    {\includegraphics[width=\imgw]{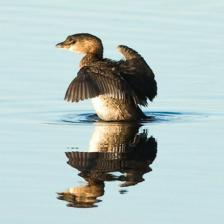}};
\node at (-1*\offset, 2*\secoffset + \textoffset) {\tiny{0.0}};

\node[inner sep=0pt] (n2) at (-1*\tabspace-\offset, 2*\secoffset)
    {\includegraphics[width=\imgw]{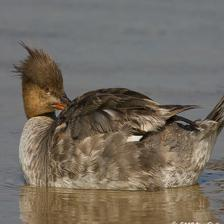}};
\node at (-1*\tabspace-\offset, \textoffset+ 2*\secoffset) {\tiny{0.0}};

\node[inner sep=0pt] (n3) at (-2*\tabspace-\offset, 2*\secoffset)
    {\includegraphics[width=\imgw]{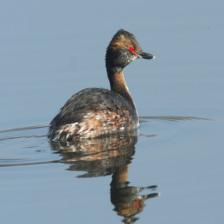}};
\node at (-2*\tabspace-\offset, \textoffset+2*\secoffset) {\tiny{0.0}};
    
\node[inner sep=0pt] (n4) at (-3*\tabspace-\offset, 2*\secoffset)
    {\includegraphics[width=\imgw]{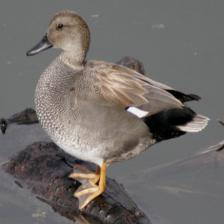}};
\node at (-3*\tabspace-\offset, \textoffset+2*\secoffset) {\tiny{0.0}};

\node[inner sep=0pt] (n5) at (-4*\tabspace-\offset, 2*\secoffset)
    {\includegraphics[width=\imgw]{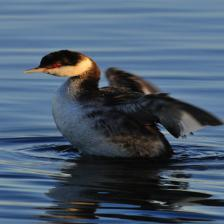}};
\node at (-4*\tabspace-\offset, \textoffset+2*\secoffset) {\tiny{0.0}};

\node at (-0.5*\offset, 2*\secoffset) {...};
\node at (-0.5*\offset, -1*\textoffset+2*\secoffset) {\tiny{Underpart color: Yellow}};

\draw [-latex](0.2*\offset, -1*\textoffset+2*\secoffset) -- (5.7, -1*\textoffset+2*\secoffset);
\node at (5.9, -1*\textoffset+2*\secoffset) {{\tiny{$+$}}};
\draw [-](-1.2*\offset, -1*\textoffset+2*\secoffset) -- (-7.7, -1*\textoffset+2*\secoffset);
\node at (-7.9, -1*\textoffset+2*\secoffset) {{\tiny{$-$}}};

% \node[inner sep=0pt] (n2) at (-5*\tabspace-\offset,0)
%     {\includegraphics[width=\imgw]{3.jpg}};

\node[inner sep=0pt] (p1) at (0, 2*\secoffset)
    {\includegraphics[width=\imgw]{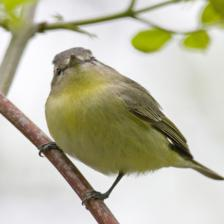}};
\node at (0, \textoffset+2*\secoffset) {\tiny{64.43}};

\node[inner sep=0pt] (p2) at (\tabspace, 2*\secoffset)
    {\includegraphics[width=\imgw]{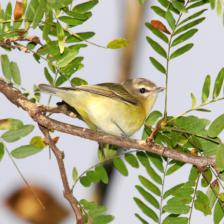}};
\node at (\tabspace, \textoffset+2*\secoffset) {\tiny{63.43}};

\node[inner sep=0pt] (p3) at (2*\tabspace, 2*\secoffset)
    {\includegraphics[width=\imgw]{figures/cub_example_sizeverysmall/pos/has_sizevery_small_(3_-_5_in)_2_47.76.jpg}};
\node at (2*\tabspace, \textoffset+2*\secoffset) {\tiny{47.76}};
    
\node[inner sep=0pt] (p4) at (3*\tabspace, 2*\secoffset)
    {\includegraphics[width=\imgw]{figures/cub_example_sizeverysmall/pos/has_sizevery_small_(3_-_5_in)_1_47.92.jpg}};
\node at (3*\tabspace, \textoffset+2*\secoffset) {\tiny{47.92}};

\node[inner sep=0pt] (p5) at (4*\tabspace, 2*\secoffset)
    {\includegraphics[width=\imgw]{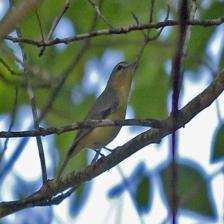}};
\node at (4*\tabspace, \textoffset+2*\secoffset) {\tiny{63.43}};

\end{tikzpicture}
% \end{document}
